# Supplementary material for: Long-Term Employment Effects of the Minimum Wage in Germany: New Data and Estimators
Source: arXiv:2310.15964 source file (2023-10-24)
Supplement: Supplementary file 1 [file Appendix_B.tex]

\section*{Appendix B $\rightarrow$ Only for us}

 \begin{figure}[h!] \caption{Effect of the minimum wage and its raises in 2017 and 2019 on employment and the SES 2014} \label{fig:event_raises1719_VSE14_old_controls}
	\begin{subfigure}{0.5\textwidth}
		\subcaption{Dependent employment} \label{fig:svgeb_raises1719_VSE14}\includegraphics[scale=0.18, trim=0 0 0 0, clip]{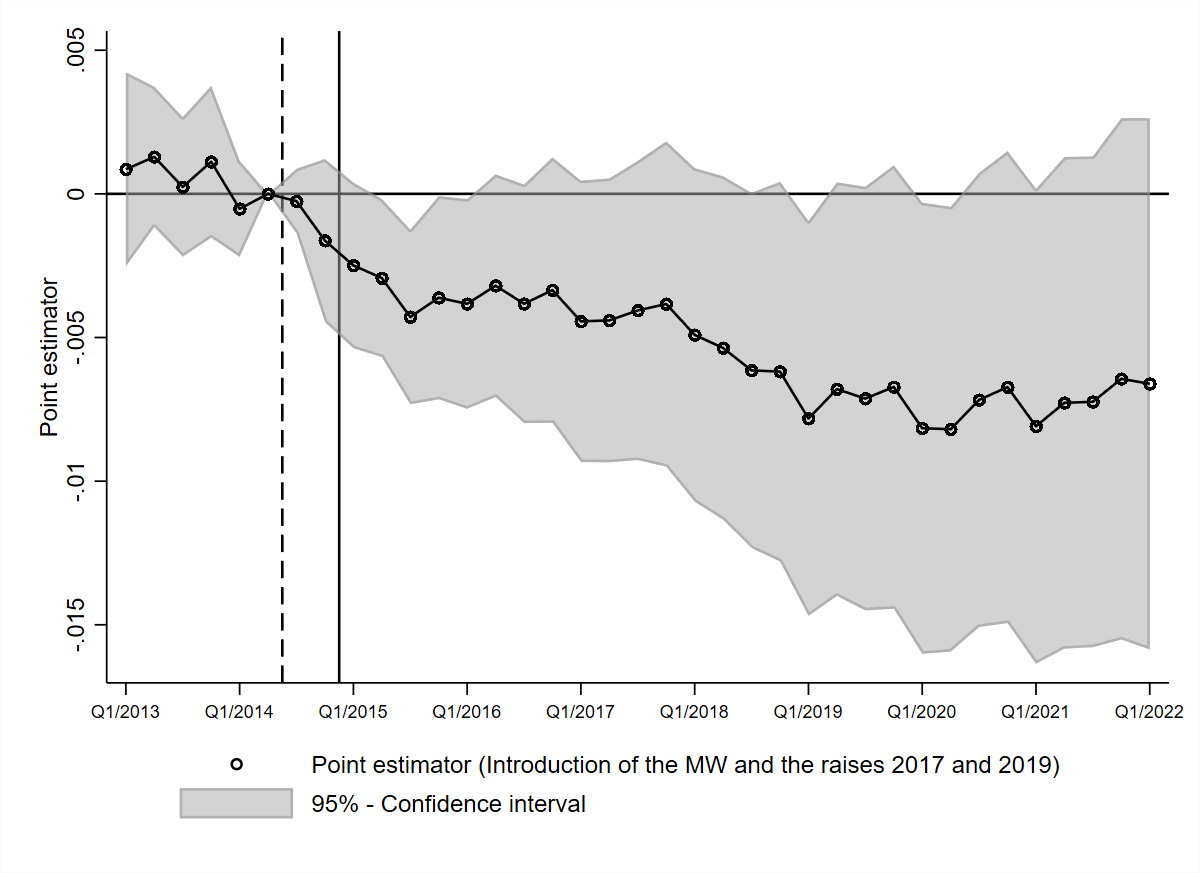}
	\end{subfigure}
	\begin{subfigure}{0.5\textwidth} 
		\subcaption{Employment subject to SSC} \label{fig:svb_raises1719_VSE14}\includegraphics[scale=0.18, trim=0 0 0 0, clip]{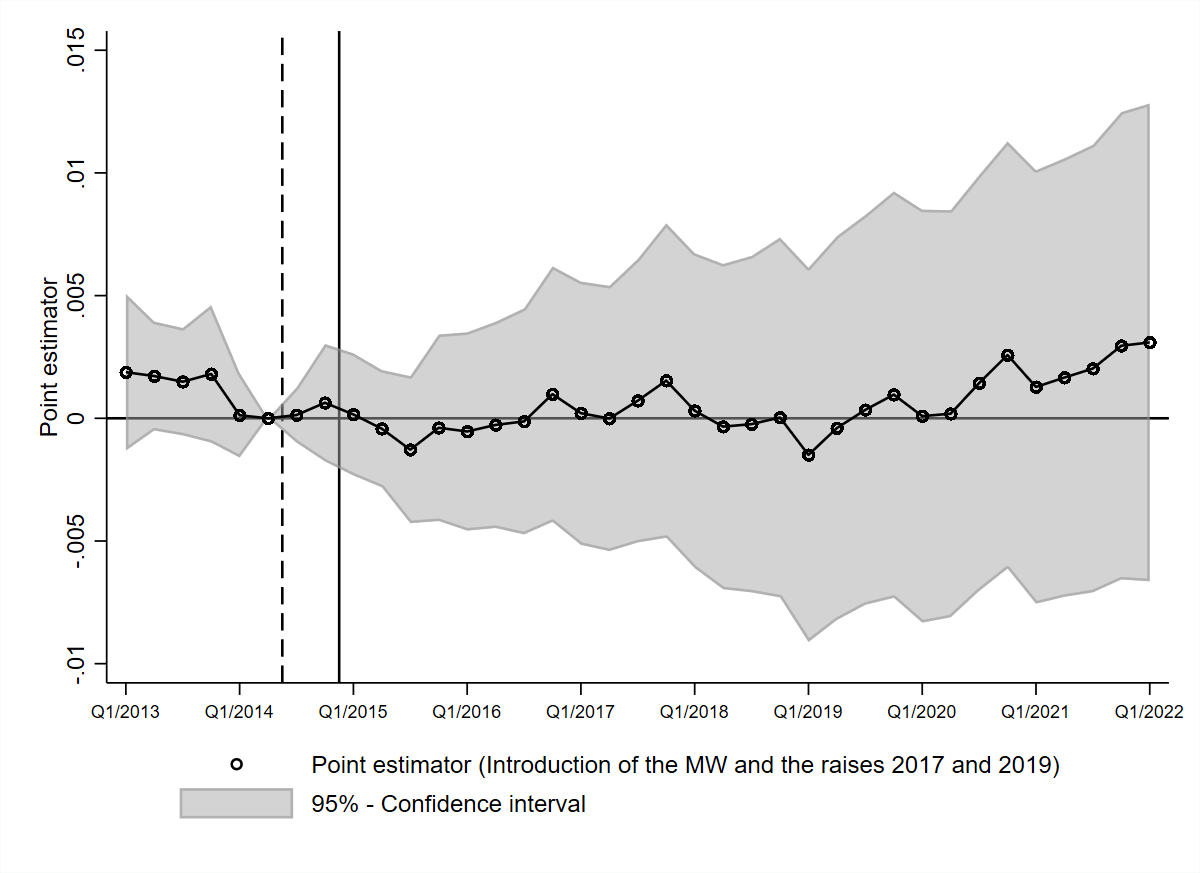}
	\end{subfigure}
 \\
         \center
	\begin{subfigure}{0.5\textwidth} 
		\subcaption{Marginal employment} \label{fig:geb_raises1719_VSE14}\includegraphics[scale=0.18, trim=0 0 0 0, clip]{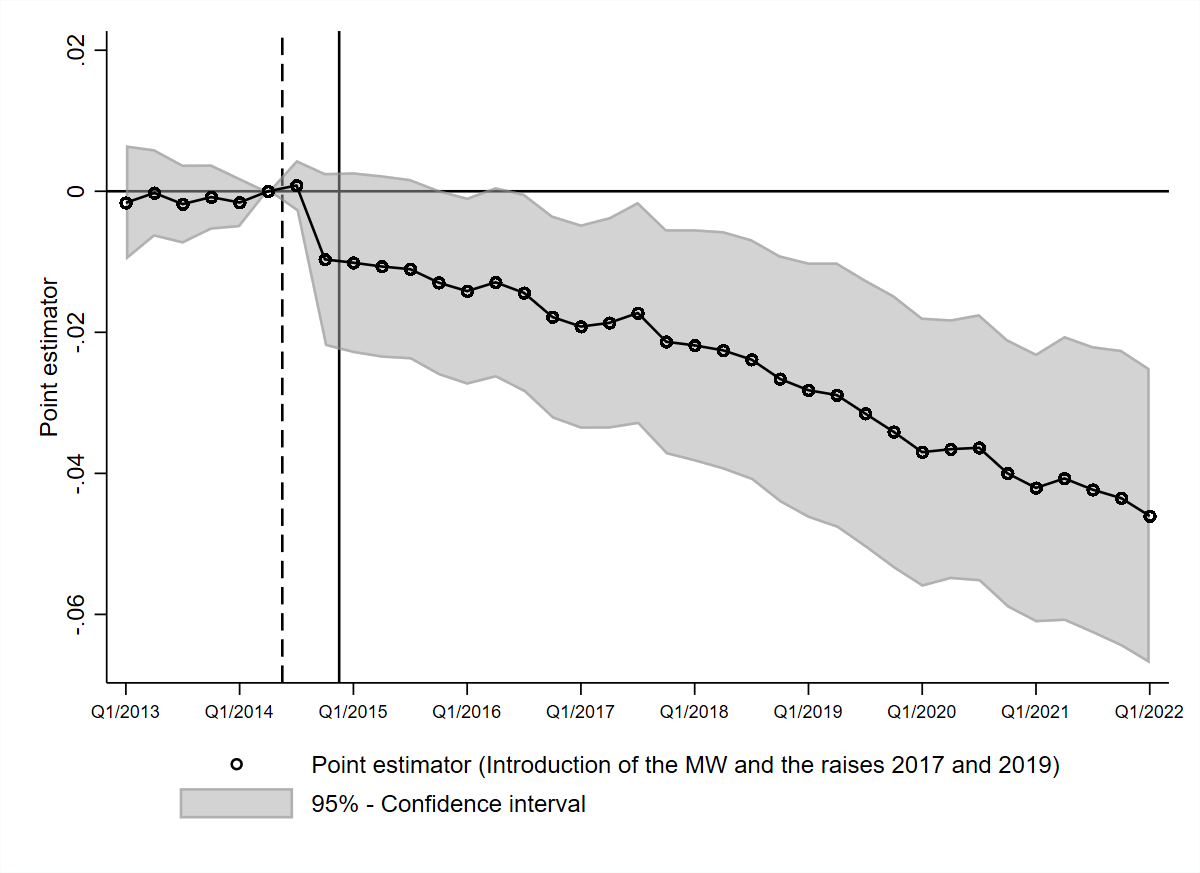}
	\end{subfigure}

	\caption*{\footnotesize Source: Statistic of the Federal Employment Agency, SES 2014; own calculations. Note: The vertical lines show the points of time when the minimum wage law was passed (August 2014), when it was introduced (January 1, 2015) as well as the points of time of the first and second increase of the minimum wage (January 1, 2017, and January 1, 2019, respectively). The point estimates and confidence intervals refer to the vector $\beta$ in equation \ref{eq:equation2}.}
\end{figure}

  \begin{figure}[h!] \caption{Effect of the minimum wage and its raises in 2017 and 2019 on employment and the SES 2014 and 2018} \label{fig:event_raises1719_VSE1418}
	\begin{subfigure}{0.5\textwidth}
		\subcaption{Dependent employment} \label{fig:svgeb_raises1719_VSE1418}\includegraphics[scale=0.18, trim=0 0 0 0, clip]{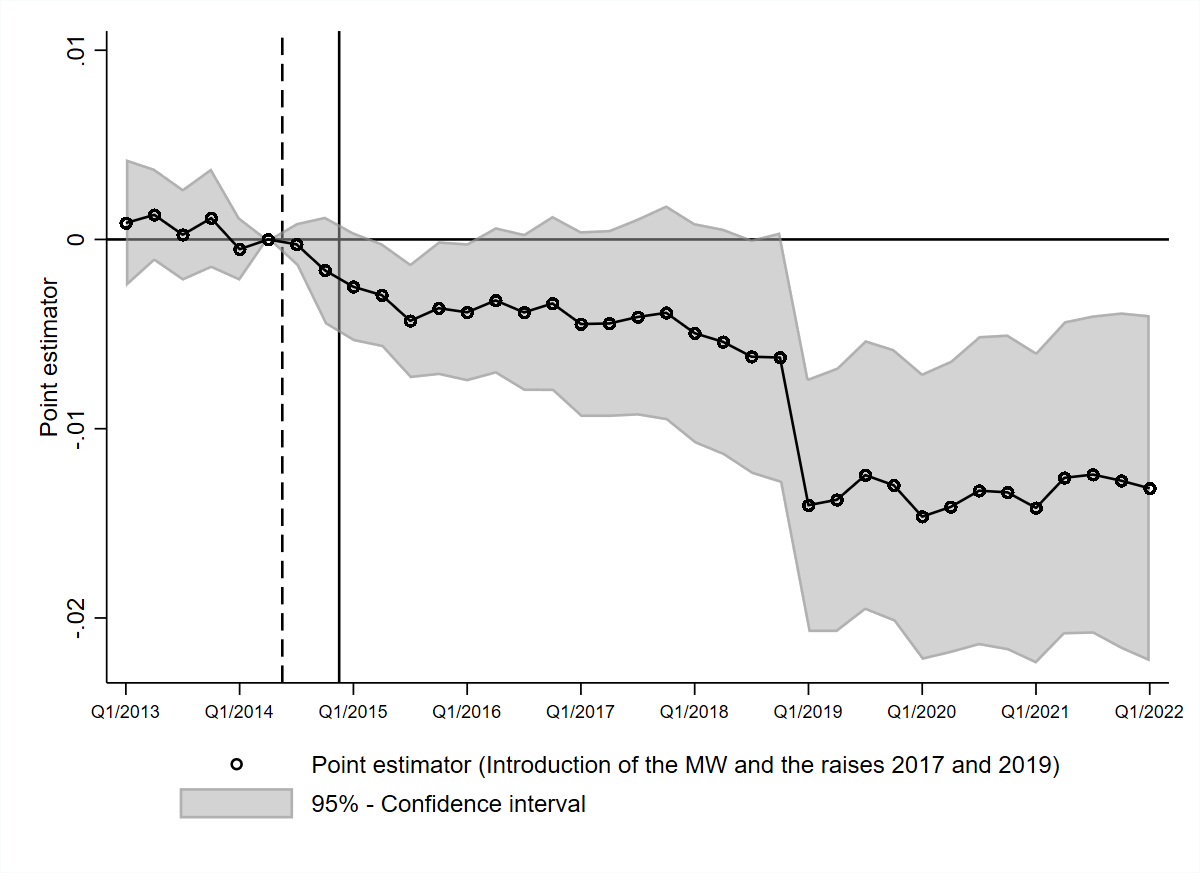}
	\end{subfigure}
	\begin{subfigure}{0.5\textwidth} 
		\subcaption{Employment subject to SSC} \label{fig:svb_raises1719_VSE1418}\includegraphics[scale=0.18, trim=0 0 0 0, clip]{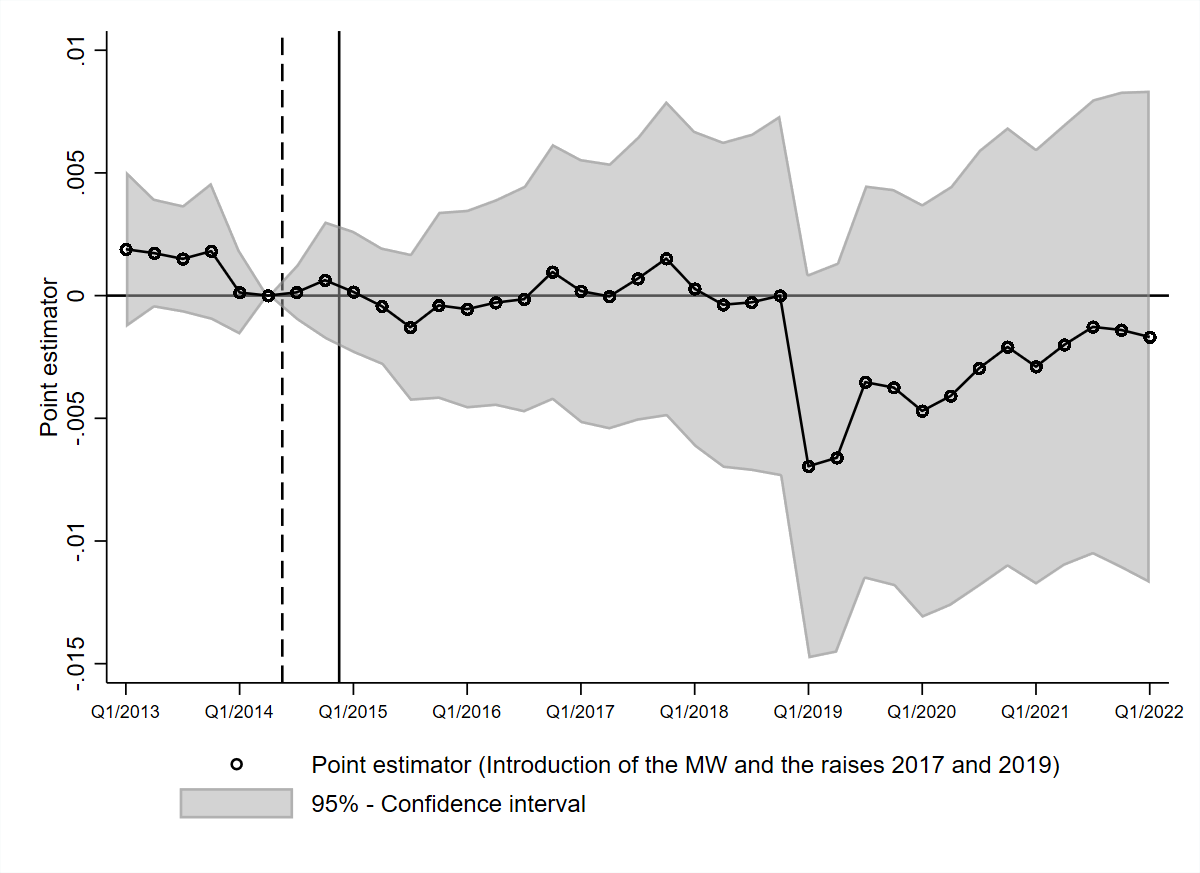}
	\end{subfigure}
 \\
         \center
	\begin{subfigure}{0.5\textwidth} 
		\subcaption{Marginal employment} \label{fig:geb_raises1719_VSE1418}\includegraphics[scale=0.18, trim=0 0 0 0, clip]{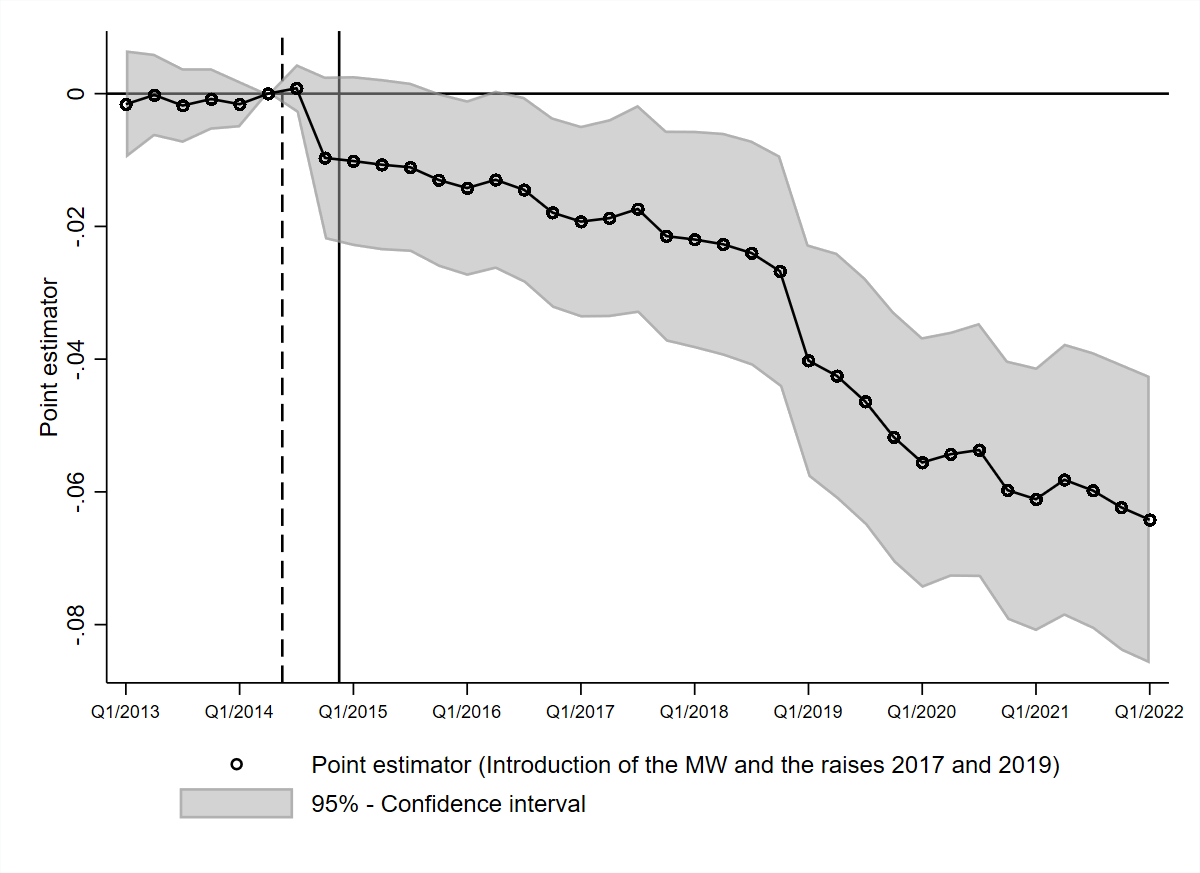}
	\end{subfigure}

	\caption*{\footnotesize Source: Statistic of the Federal Employment Agency, SES 2014; own calculations. Note: The vertical lines show the points of time when the minimum wage law was passed (August 2014), when it was introduced (January 1, 2015) as well as the points of time of the first and second increase of the minimum wage (January 1, 2017, and January 1, 2019, respectively). The point estimates and confidence intervals refer to the vector $\beta$ in equation \ref{eq:equation2}.}
\end{figure}

  \begin{figure}[h!] \caption{Effect of the minimum wage and its raises in 2017 and 2019 on employment} \label{fig:event_raises1719}
	\begin{subfigure}{0.5\textwidth}
		\subcaption{Dependent employment} \label{fig:svgeb_raises1719}\includegraphics[scale=0.18, trim=0 0 0 0, clip]{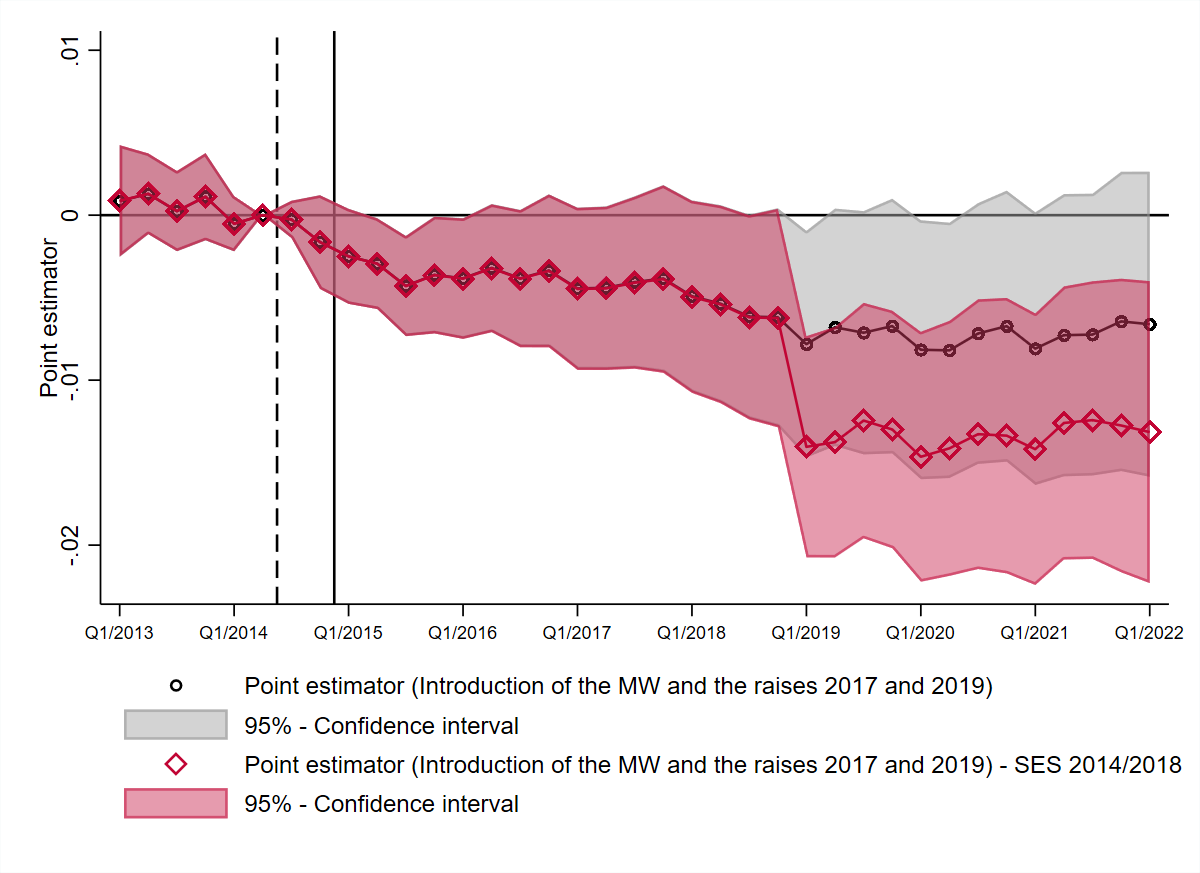}
	\end{subfigure}
	\begin{subfigure}{0.5\textwidth} 
		\subcaption{Employment subject to SSC} \label{fig:svb_raises1719}\includegraphics[scale=0.18, trim=0 0 0 0, clip]{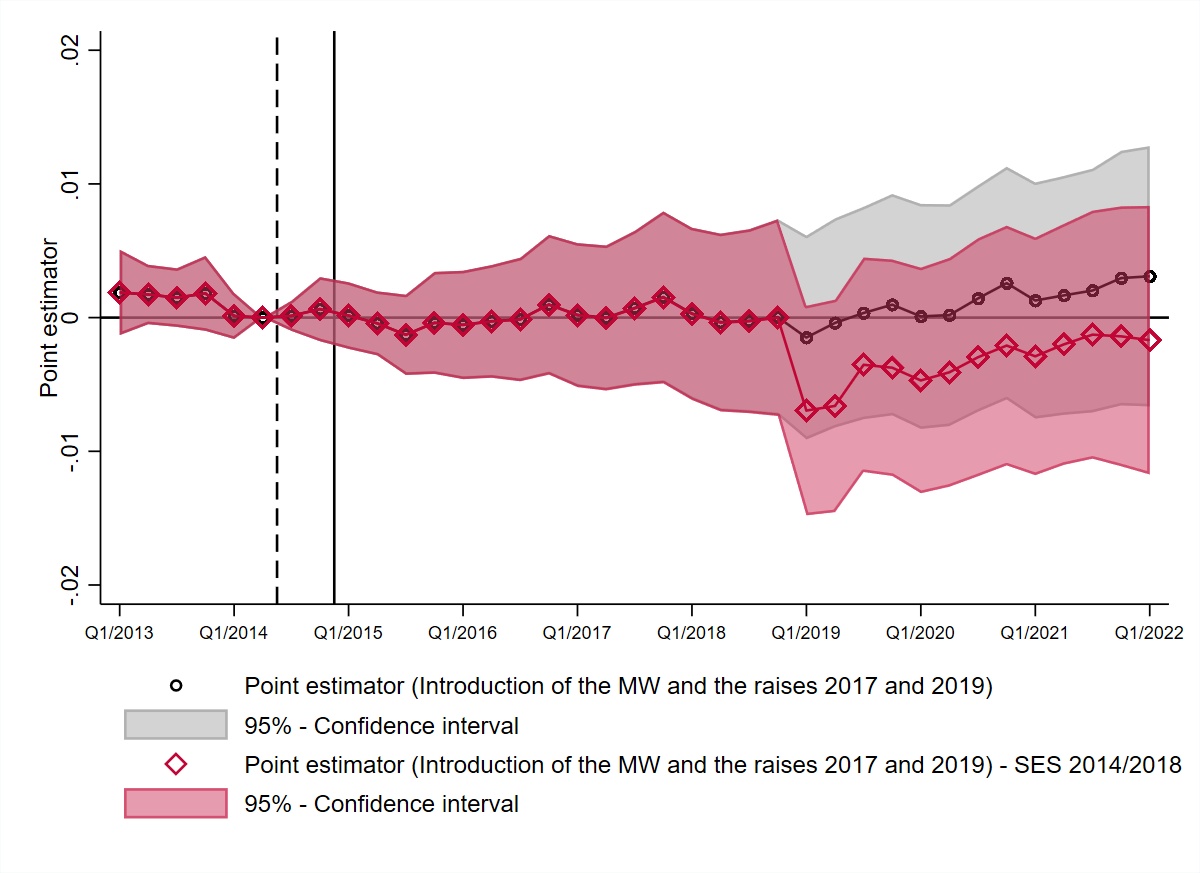}
	\end{subfigure}
 \\
         \center
	\begin{subfigure}{0.5\textwidth} 
		\subcaption{Marginal employment} \label{fig:geb_raises1719}\includegraphics[scale=0.18, trim=0 0 0 0, clip]{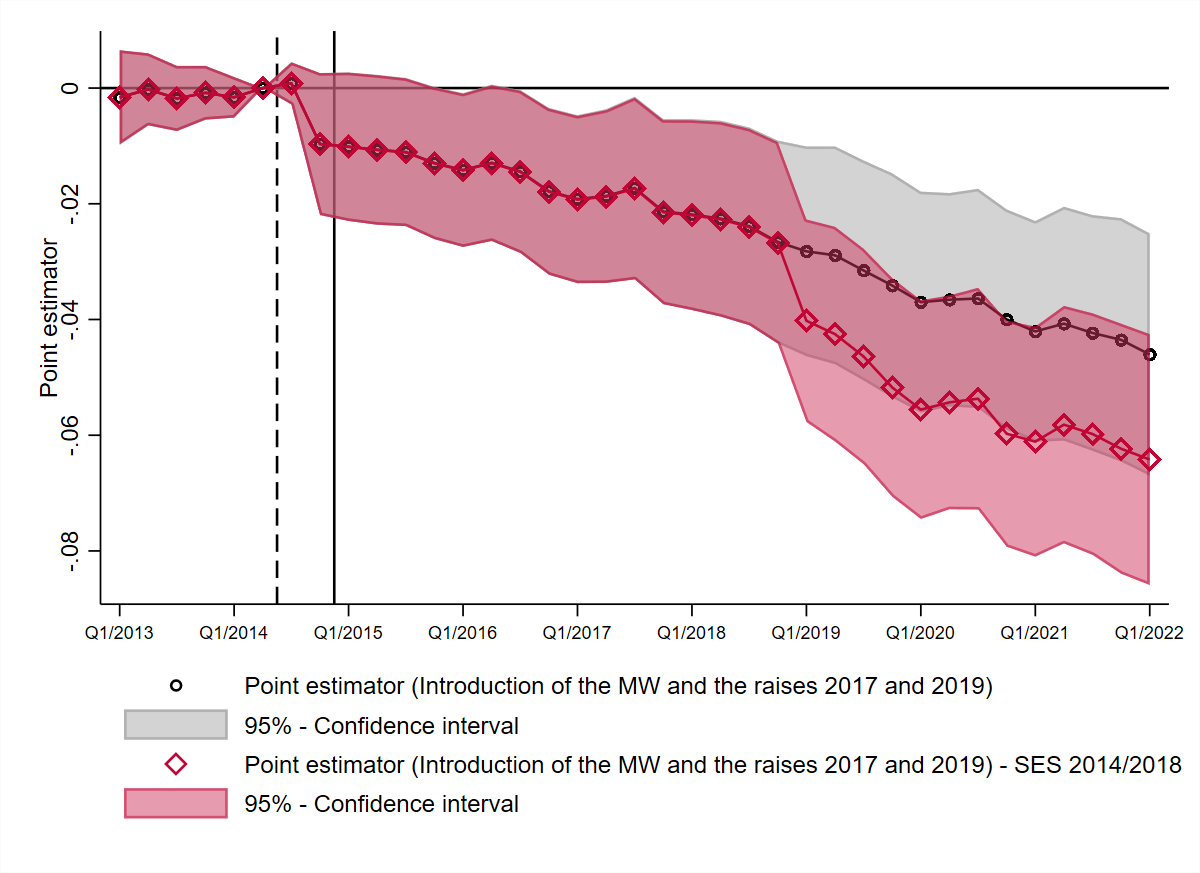}
	\end{subfigure}

	\caption*{\footnotesize Source: Statistic of the Federal Employment Agency, SES 2014; own calculations. Note: The vertical lines show the points of time when the minimum wage law was passed (August 2014), when it was introduced (January 1, 2015) as well as the points of time of the first and second increase of the minimum wage (January 1, 2017, and January 1, 2019, respectively). The point estimates and confidence intervals refer to the vector $\beta$ in equation \ref{eq:equation2}.}
\end{figure}

  \begin{figure}[h!] \caption{Effect of the minimum wage and its raises on employment} \label{fig:event_raises}
	\begin{subfigure}{0.5\textwidth}
		\subcaption{Dependent employment} \label{fig:svgeb_raises}\includegraphics[scale=0.18, trim=0 0 0 0, clip]{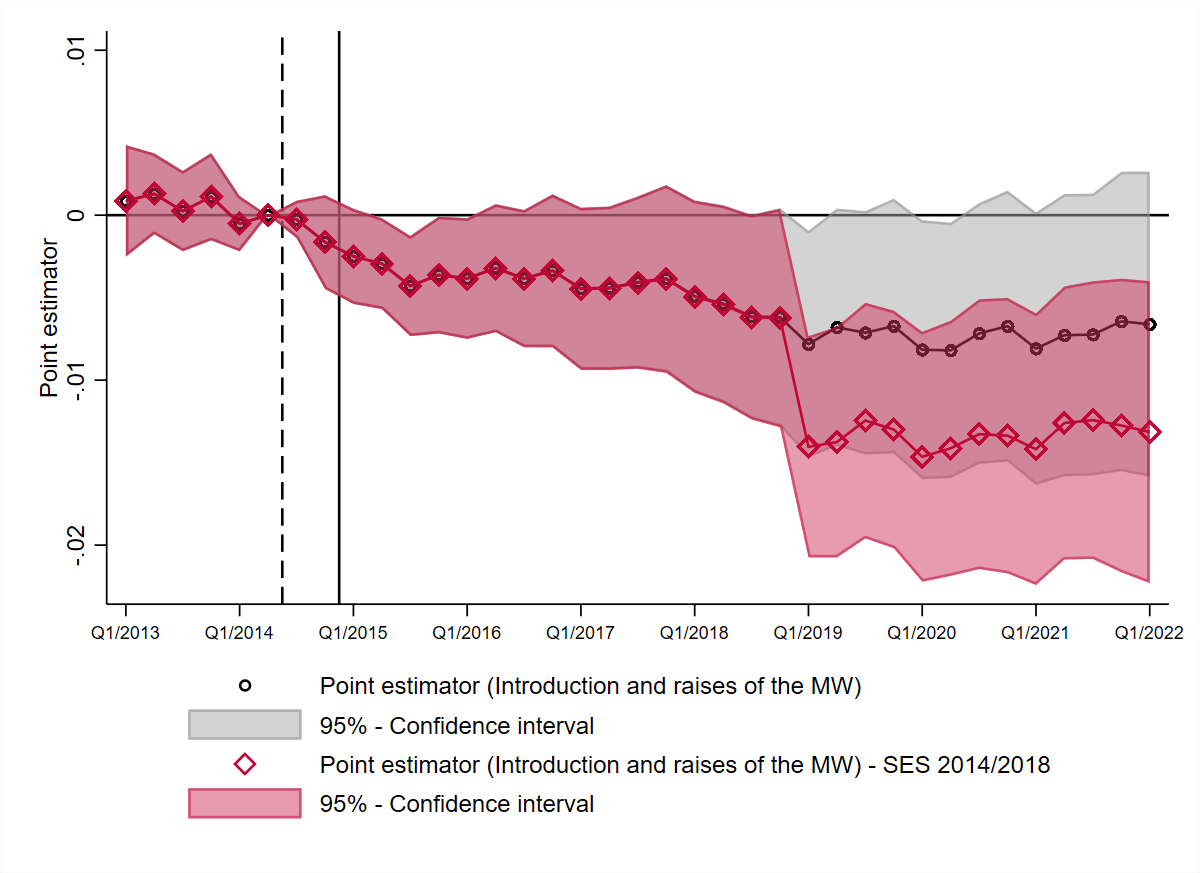}
	\end{subfigure}
	\begin{subfigure}{0.5\textwidth} 
		\subcaption{Employment subject to SSC} \label{fig:svb_raises}\includegraphics[scale=0.18, trim=0 0 0 0, clip]{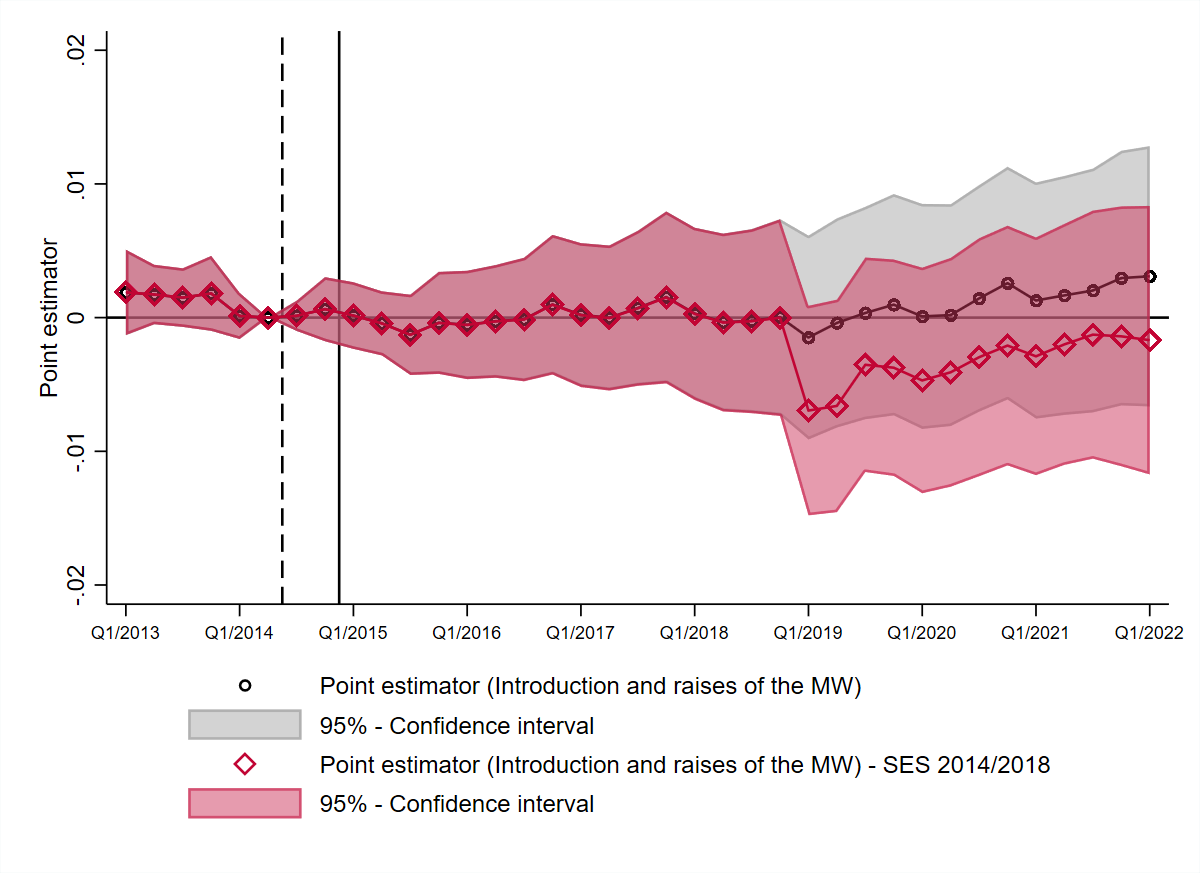}
	\end{subfigure}
 \\
         \center
	\begin{subfigure}{0.5\textwidth} 
		\subcaption{Marginal employment} \label{fig:geb_raises}\includegraphics[scale=0.18, trim=0 0 0 0, clip]{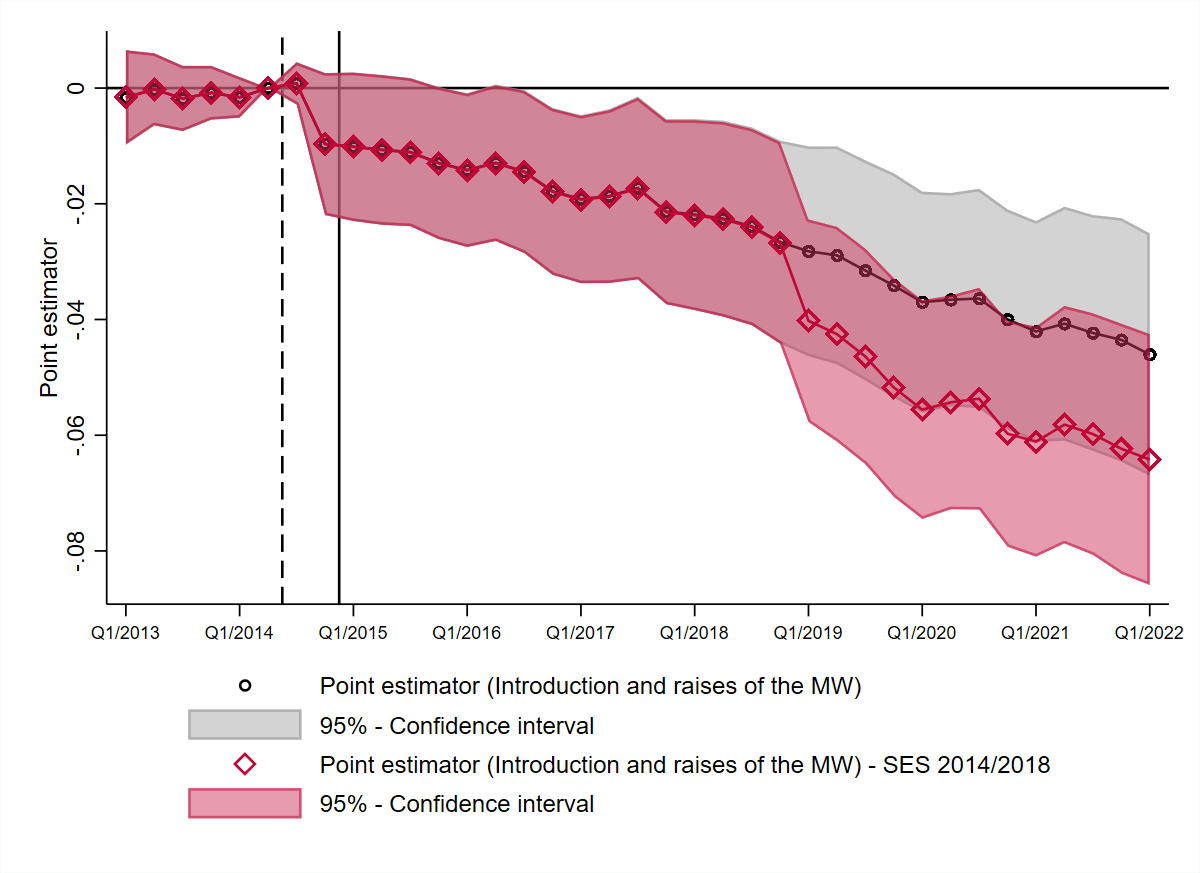}
	\end{subfigure}

	\caption*{\footnotesize Source: Statistic of the Federal Employment Agency, SES 2014; own calculations. Note: The vertical lines show the points of time when the minimum wage law was passed (August 2014), when it was introduced (January 1, 2015) as well as the points of time of the first and second increase of the minimum wage (January 1, 2017, and January 1, 2019, respectively). The point estimates and confidence intervals refer to the vector $\beta$ in equation \ref{eq:equation2}.}
\end{figure}

   \begin{figure}[h!] \caption{Effect of the minimum wage on employment for regions with a high wage gap in 2014 and 2018} \label{fig:event_groups_hh}
	\begin{subfigure}{0.5\textwidth}
		\subcaption{Dependent employment} \label{fig:svgeb_groups_hh}\includegraphics[scale=0.18, trim=0 0 0 0, clip]{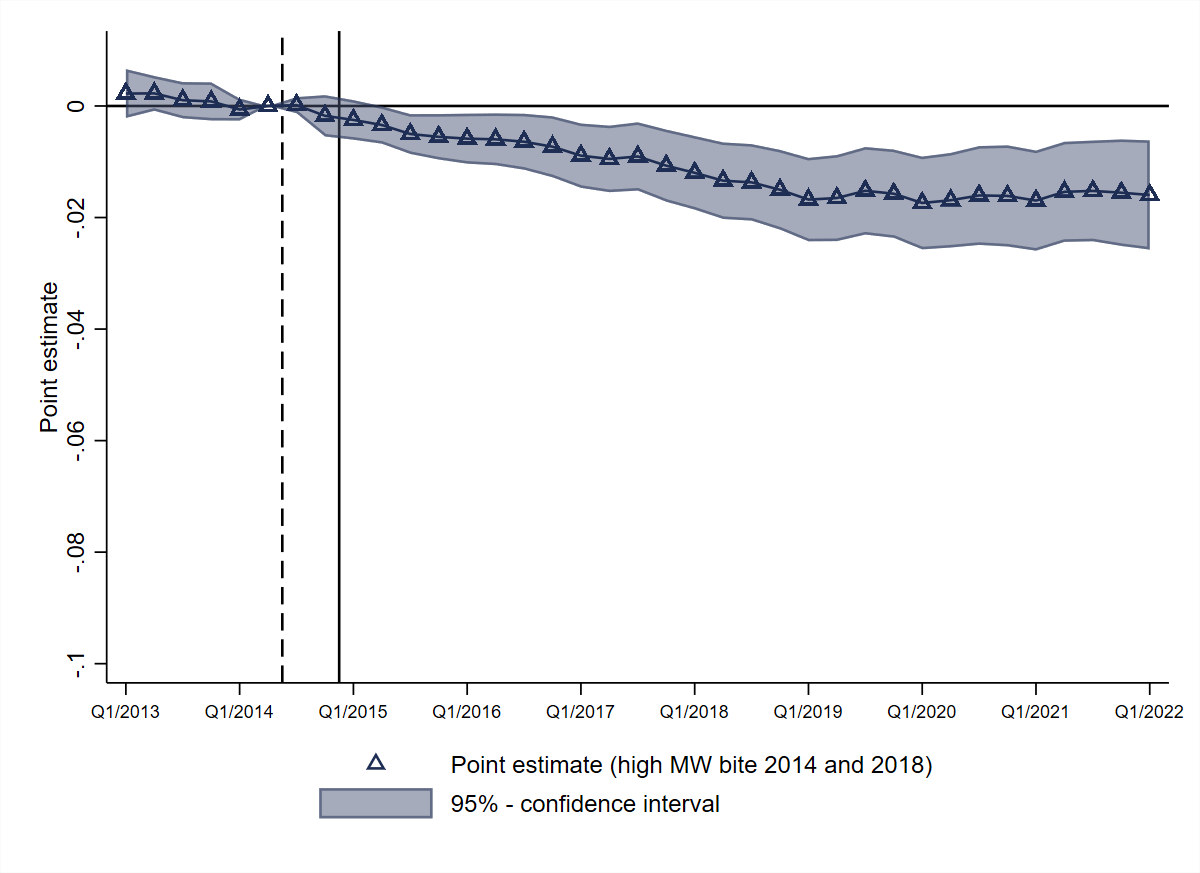}
	\end{subfigure}
	\begin{subfigure}{0.5\textwidth} 
		\subcaption{Employment subject to SSC} \label{fig:svb_groups_hh}\includegraphics[scale=0.18, trim=0 0 0 0, clip]{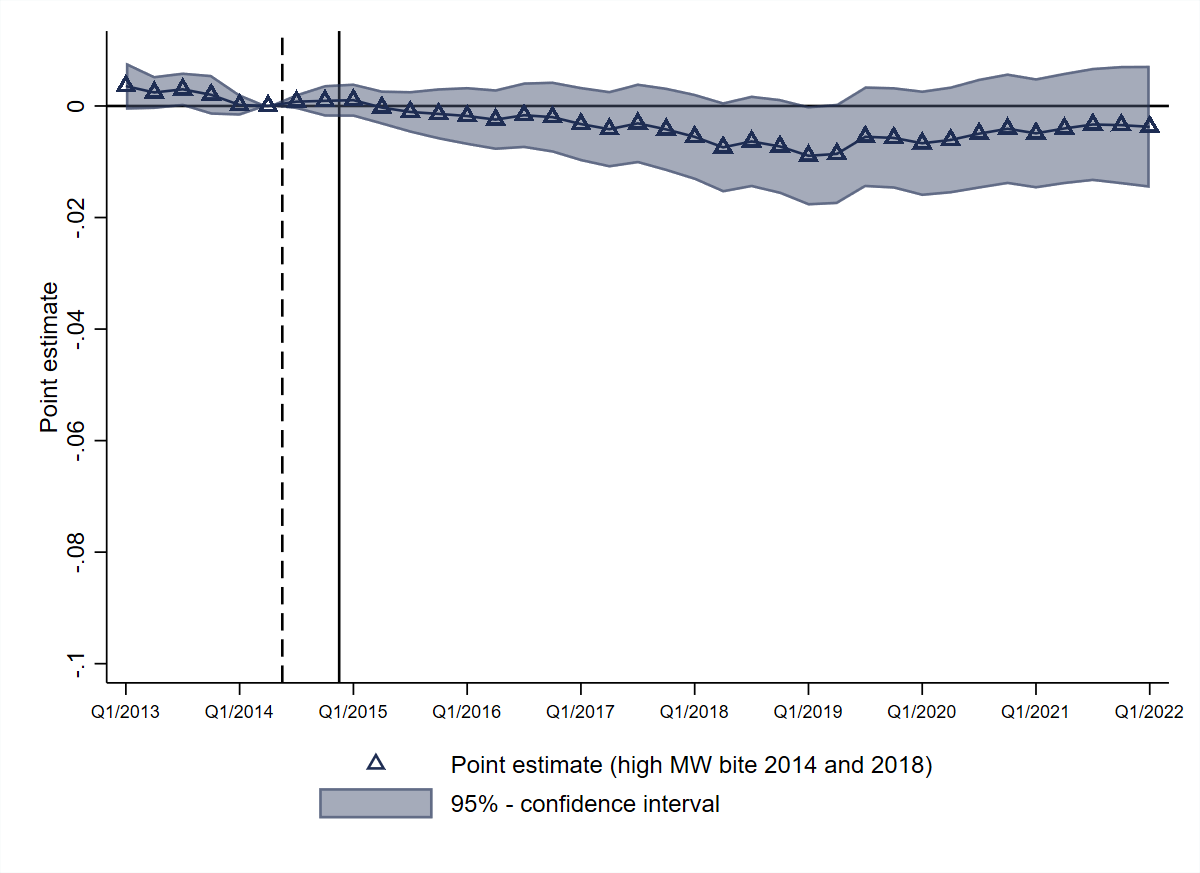}
	\end{subfigure}
 \\
         \center
	\begin{subfigure}{0.5\textwidth} 
		\subcaption{Marginal employment} \label{fig:geb_groups_hh}\includegraphics[scale=0.18, trim=0 0 0 0, clip]{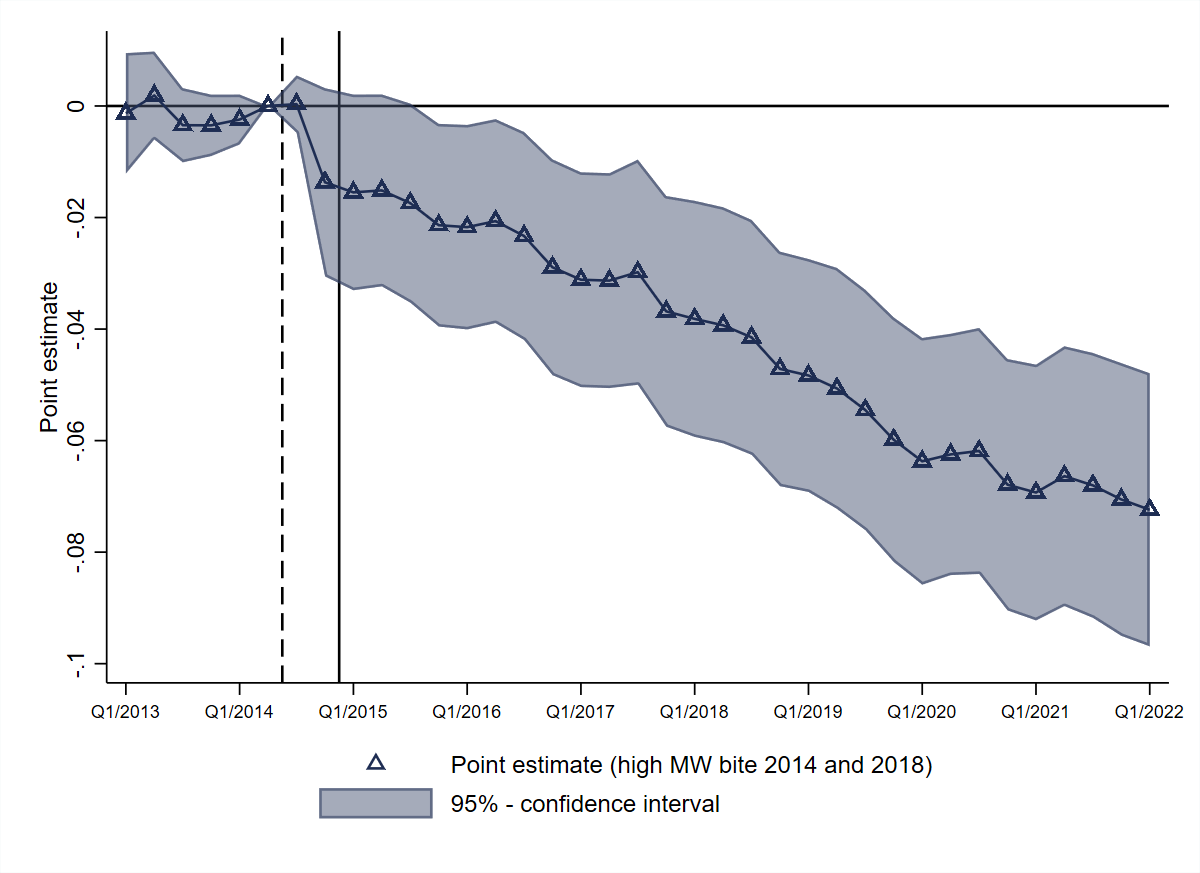}
	\end{subfigure}

	\caption*{\scriptsize Source: Statistic of the Federal Employment Agency, SES 2014, 2018; own calculations. Note: The vertical lines show the points of time when the minimum wage law was passed (August 2014) and when it was introduced (January 1, 2015). The treatment effect refers to the coefficient $\beta$ in equation \ref{eq:equation4}. The included control variables are interactions of: time, east, and population share between 18 and 64 years in 2013; time, east, and type of labour market region; time, east, and employment share in different sectors. Standard errors (in parentheses) are clustered on the level of the labour market regions.}
\end{figure}

   \begin{figure}[h!] \caption{Effect of the minimum wage on employment for regions with changing treatment in 2014 and 2018} \label{fig:event_groups_mixed}
	\begin{subfigure}{0.5\textwidth}
		\subcaption{Dependent employment} \label{fig:svgeb_groups_mixed}\includegraphics[scale=0.18, trim=0 0 0 0, clip]{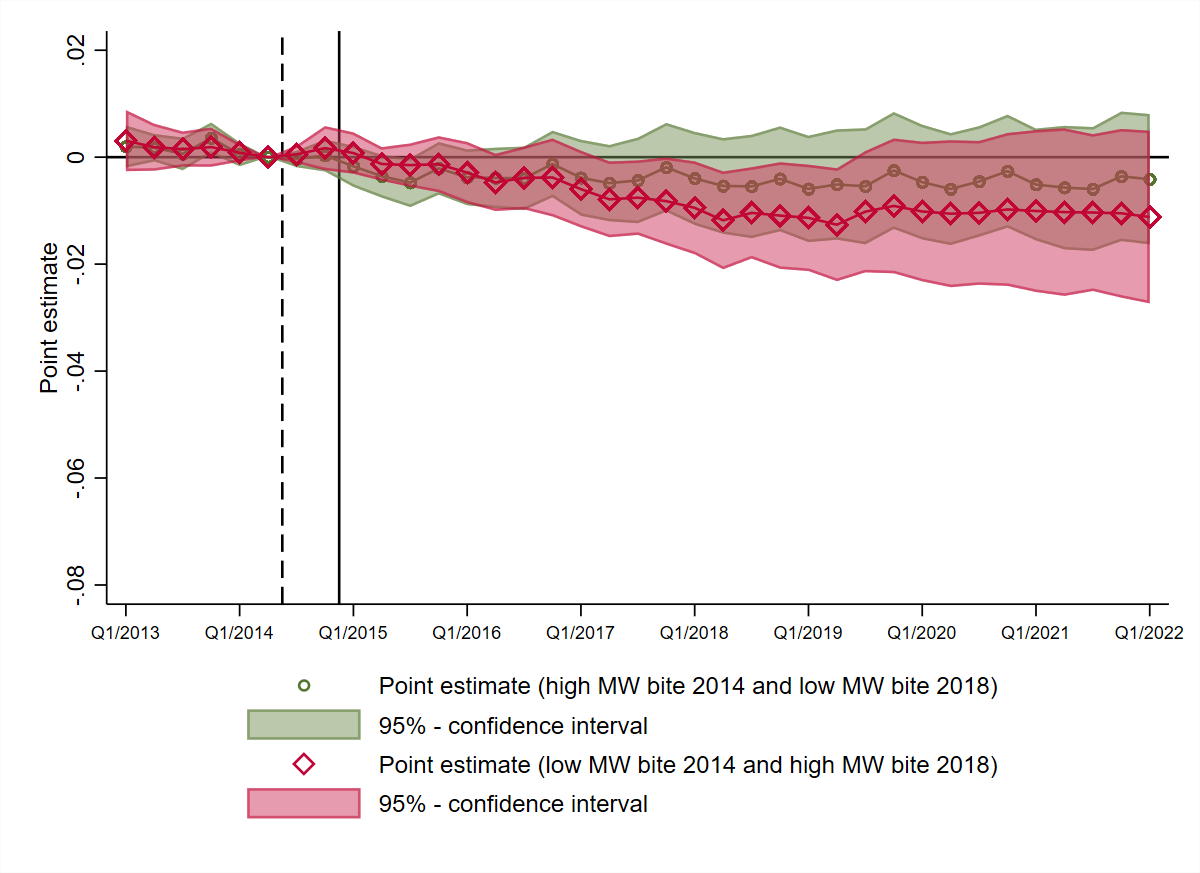}
	\end{subfigure}
	\begin{subfigure}{0.5\textwidth} 
		\subcaption{Employment subject to SSC} \label{fig:svb_groups_mixed}\includegraphics[scale=0.18, trim=0 0 0 0, clip]{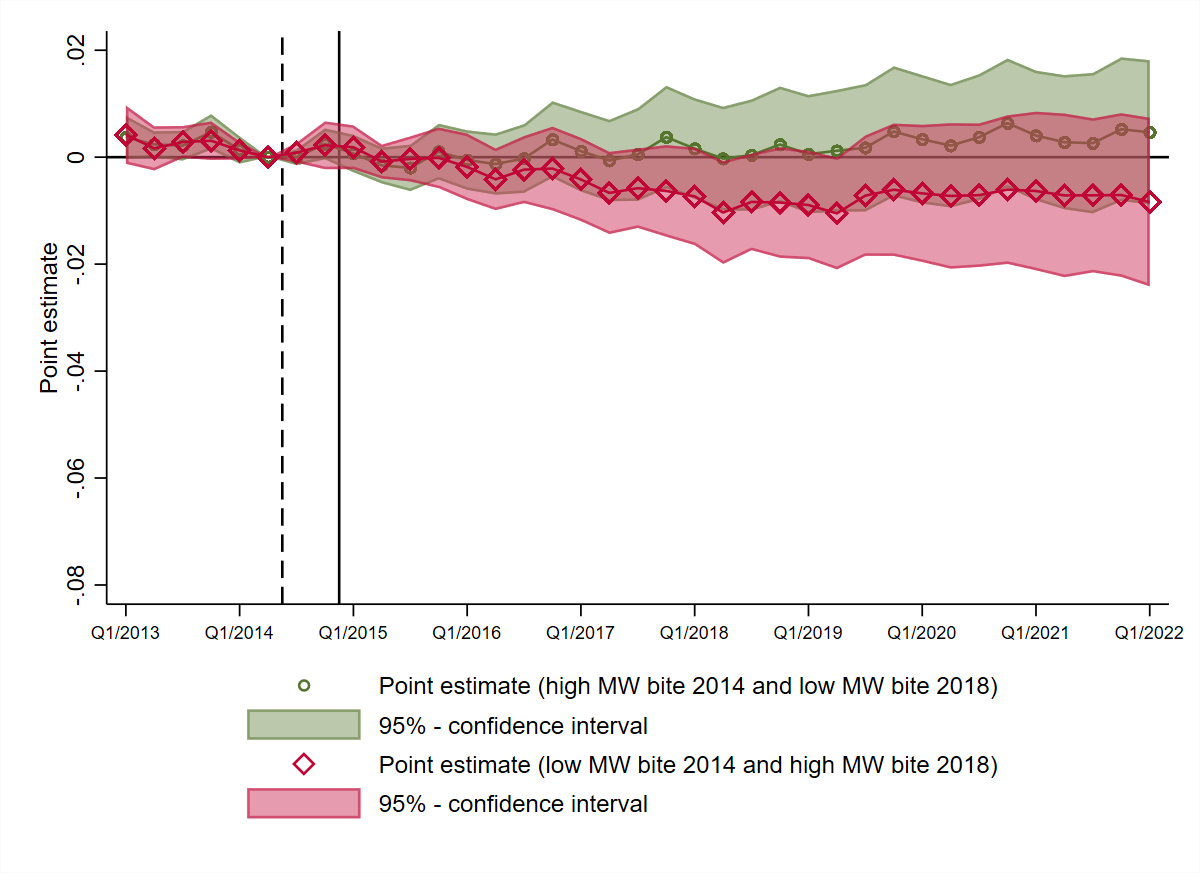}
	\end{subfigure}
 \\
         \center
	\begin{subfigure}{0.5\textwidth} 
		\subcaption{Marginal employment} \label{fig:geb_groups_mixed}\includegraphics[scale=0.18, trim=0 0 0 0, clip]{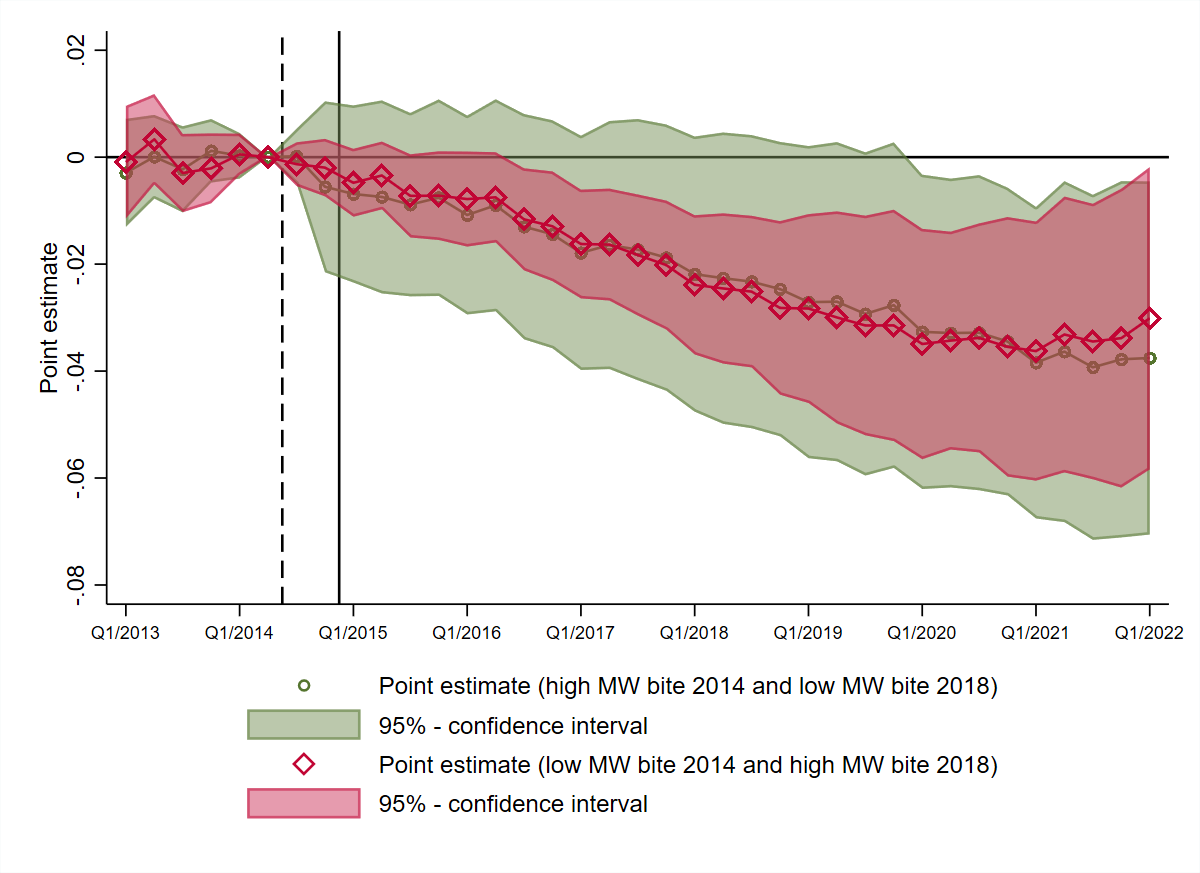}
	\end{subfigure}

	\caption*{\scriptsize Source: Statistic of the Federal Employment Agency, SES 2014, 2018; own calculations. Note: The vertical lines show the points of time when the minimum wage law was passed (August 2014) and when it was introduced (January 1, 2015). The treatment effect refers to the coefficients $\gamma$ and $\delta$ in equation \ref{eq:equation4}. The included control variables are interactions of: time, east, and population share between 18 and 64 years in 2013; time, east, and type of labour market region; time, east, and employment share in different sectors. Standard errors (in parentheses) are clustered on the level of the labour market regions.}
\end{figure}

 \begin{scriptsize}
	% Table generated by Excel2LaTeX from sheet 'Incremental_1418_BIP'
\begin{table}[htbp]
  \centering
 \caption{Effects of the minimum wage introduction and its raises on regional employment \textbf{With ``GDP per capita x quarter'' as additional control}}
  \label{tab:incremental_VSE1418_allRaises_bip}
    \begin{tabular}{lccc}
    \toprule
    \toprule
    \multicolumn{1}{l}{} & (1)   & (2)  & (3) \\
    \multicolumn{1}{l}{VARIABLES} & Dependent  & Employment  & Marginal  \\
   & employment  & subject to SSC  & employment  \\
    \midrule
    \multicolumn{1}{l}{} &       &       &  \\
    \multicolumn{1}{l}{Treatment 2014   } & -0.00295** & -0.000136 & -0.0112* \\
    \multicolumn{1}{l}{} & (0.00144) & (0.00152) & (0.00589) \\
    \multicolumn{1}{l}{Placebo} & 0.000601 & 0.00142 & -0.00125 \\
    \multicolumn{1}{l}{} & (0.00111) & (0.00107) & (0.00245) \\
    \multicolumn{1}{l}{Treatment 2014 x (Time $>$ 2016)} & -0.00250 & 0.00151 & -0.0171*** \\
    \multicolumn{1}{l}{} & (0.00251) & (0.00256) & (0.00499) \\
    \multicolumn{1}{l}{Treatment 2018 x (Time $>$ 2018)} & -0.00773*** & -0.00627*** & -0.0181*** \\
    \multicolumn{1}{l}{} & (0.00236) & (0.00240) & (0.00545) \\
    \multicolumn{1}{l}{Treatment 2018 x (Time $>$ 2019)} & -0.000188 & 0.000870 & -0.00580*** \\
    \multicolumn{1}{l}{} & (0.00113) & (0.00115) & (0.00216) \\
    \multicolumn{1}{l}{Treatment 2018 x (Time $>$ 2020)} & 0.000748 & 0.000969 & -0.000631 \\
    \multicolumn{1}{l}{} & (0.000966) & (0.00102) & (0.00246) \\
    \multicolumn{1}{l}{Treatment 2018 x (Time $>$ 2021)} & -0.000849 & -0.000882 & -0.000636 \\
    \multicolumn{1}{l}{} & (0.000654) & (0.000688) & (0.00189) \\
    %\multicolumn{1}{l}{Constant} & 12.58*** & 12.06*** & 10.87*** \\
    %\multicolumn{1}{l}{} & (0.574) & (0.570) & (1.106) \\
    %\multicolumn{1}{l}{} &       &       &  \\
    \midrule
    \multicolumn{1}{l}{Observations} & 9,509 & 9,509 & 9,509 \\
    \multicolumn{1}{l}{R$^{2}$ (within)} & 0.605 & 0.588 & 0.500 \\
    \midrule
    \multicolumn{1}{l}{Labour market region FE} & X     & X     & X \\
    \multicolumn{1}{l}{Quarter FE} & X     & X     & X \\
    \multicolumn{1}{l}{Controls} & X     & X     & X \\
    \bottomrule
    \bottomrule
    \end{tabular}%
\caption*{\scriptsize Source: Statistic of the Federal Employment Agency, SES 2014, 2018; own calculations. Note: The treatment effects refer to the coefficients $\beta$, $\delta_{2016}$, and $\delta_{\tau}$ in Equation (\ref{eq:equation3}). The binary treatment 2014 (2018) equals 1 if the regional wage gap in 2014 (2018) is equal to or above the population-weighted median. The control variables included are interactions of: time, east, and population share between 18 and 64 years in 2013; time, east, and type of labour market region; time, east, and employment share in different sectors; time and GDP per capita in 2013. Standard errors (in parentheses) are clustered at the level of the labour market regions. Confidence level: ***p$<$0.01, **p$<$0.05, *p$<$0.1.}
\end{table}%

 \end{scriptsize}
